# Supplementary material for: LightMem: Lightweight and Efficient Memory-Augmented Generation
Source: arXiv:2510.18866 source file (2026-02-28)
Supplement: Supplementary file 1 [file appendix_lightmem_results.tex]

\section{Lightmem Results}
\label{lightmem_results}

We present the numerical results of the effects of LightMem parameters (compression ratio and STM threshold) on the final performance in the following tables, which correspond to online soft update and offline update, respectively.
