# Supplementary material for: LightMem: Lightweight and Efficient Memory-Augmented Generation
Source: arXiv:2510.18866 source file (2026-02-28)
Supplement: Supplementary file 2 [file cost_appendix.tex]

\begin{table}[htbp]
\centering
\caption{\textbf{Cost of Retrieval-Augmented Responses}. Average end-to-end time (seconds) for \emph{Search + Answer} per query. \textit{Full Text} has no retrieval, so the time reflects answer latency only.}
\label{tab:rag_cost_time}

\setlength{\tabcolsep}{5pt}
\scriptsize
\begin{tabular}{@{}lcc@{}}
\toprule
\multirow{2}{*}{\textbf{Method}} & \multicolumn{2}{c}{\textbf{Avg Time (s)}} \\
\cmidrule(lr){2-3}
& \cellcolor{gptgray}\textbf{\openailogo GPT-4o-mini} & \cellcolor{qwenlav}\textbf{\qwenlogo Qwen3-30B-A3B-Instruct-2507} \\
\midrule
\textit{Full Text} & \cellcolor{gptgray} 11.50 & \cellcolor{qwenlav}-- \\
\textit{Naive RAG} & \cellcolor{gptgray}6.57 & \cellcolor{qwenlav} 5.50 \\
\textit{LangMem} & \cellcolor{gptgray}-- & \cellcolor{qwenlav}-- \\
\textit{A-MEM} & \cellcolor{gptgray}-- & \cellcolor{qwenlav}-- \\
\textit{MemoryOS} & \cellcolor{gptgray} 2.15 & \cellcolor{qwenlav} 1.64 \\
\textit{Mem0} & \cellcolor{gptgray} 8.77 & \cellcolor{qwenlav} 7.80 \\
\textit{LightMem} & \cellcolor{gptgray}-- & \cellcolor{qwenlav}-- \\
\bottomrule
\end{tabular}
\end{table}
